# Supplementary material for: Accurate relativistic chiral nucleon-nucleon interaction up to NNLO
Source: arXiv:2111.07766 source file (2022-03-24)
Supplement: Supplementary file 1 [file Supplementary_Material_V1.pdf]

# Supplementary Material for "Accurate relativistic chiral nucleon-nucleon interaction up to NNLO"

In this supplemental material, we provide further details that are useful to understand the results presented in the main text.

## FITS WITH 17 LECS

In this section, we present the $NN$ scattering phase shifts obtained in our NNLO chiral nuclear force with 17 LECs as dictated in Ref. [1], and explain why two nominal N$^3$LO contact terms need to be promoted.

Following the same fitting strategy as detailed in the main text, we obtain the results shown in Fig. 1. For comparison, we also show the non-relativistic NNLO and N$^3$LO results which are referred to as "NR-NNLO" [2], "NR-N$^3$LO-Idaho" [3, 4], and "NR-N$^3$LO-EKM" [5, 6], respectively. In Table. I, we tabulate the $\tilde{\chi}^2$ obtained by fitting to the PWA93 phase shifts at laboratory energies $T_{\rm lab} = 1, 5, 10, 25, 50, 100, 150, 200$ MeV for each partial wave, as well as the sum of them. Clearly, compared to the results shown in the main text, only the $^3P_2$ partial wave cannot be satisfactorily described.

It was already noticed in Ref. [2] that the non-relativistic subleading TPE potential is a bit strong such that the description of the phase shifts can be worsened at NNLO for some partial waves, e.g., the $^3P_2$ partial wave. This was attributed to the dimensional regularization applied in regularizing the TPE loop diagrams that takes into account the high-momentum contribution of pion loops. Replacing the dimensional regularization with the so-called spectrum functional regularization, which is essentially a cutoff regularization, improves the description of $^3P_2$ at NNLO (but worsens the description of some other partial waves [7–9]). On the other hand, a better description with the dimensional regularization can be obtained when the non-relativistic chiral potential was constructed up to N$^3$LO [3], which yields results in good agreement with the PWA93 phase shifts for all the partial waves considered there (but with a dedicate fine-tuning of the NLO $\pi N$ LECs $c_2$ and $c_4$). In Refs. [5, 10], the authors presented another high-quality non-relativistic chiral potential with NLO $\pi N$ LECs $c_i$'s fixed using an appropriate regularization in coordinate space. In addition, since there is no LEC to balance the large TPE contributions except the cutoff and the NLO LECs of $\pi N$ scattering $c_1, c_2, c_3, c_4$, $V_{\rm TPE}^{\rm NNLO}$ introduces strong cutoff dependence for the partial waves with orbital angular momentum $L = 2$, particularly, $^3D_3$. This problem can be alleviated after the non-relativistic chiral potential is constructed up to N$^3$LO in which new LECs are introduced.

In our study, we find that the relativistic potential also suffers from the two problems mentioned above but to a less extent. The contributions from the relativistic $V_{\rm TPE}^{\rm NNLO}$ is large and compatible with (but smaller than) their corresponding non-relativistic counterparts [11].

The large subleading TPE contributions force the $^3P_2$ phase shifts to drop down with increasing $T_{\rm lab}$. To compensate them, we promote two of the higher order contact terms to NLO for the $^3P_2$-$^3F_2$ coupled channel, which is equivalent to breaking the correlations between the $J = 2$ partial waves. In the following we explain in detail how we achieved this.

In our covariant power counting scheme [1], the NLO contact terms for the $J = 2$ partial waves already contain nominally higher order contact terms (in the language of HBChPT) as is explicitly exhibited in Eq. (22). Obviously, for the two $D$-waves, at this order, the contact terms are counted nominally as of $\mathcal{O}(p^4)$. For $^3P_2$, the first term is counted as of order $\mathcal{O}(p^2)$, while the other two terms are of order $\mathcal{O}(p^4)$ and $\mathcal{O}(p^6)$, respectively. The situation is similar for $^3F_2$ and the off-diagonal $^3P_2$-$^3F_2$. This way, we have in total eight different structures, corresponding to eight combinations of the NLO LECs($O_{5,\ldots,17}$) for all the $J = 2$ partial waves, while only three of them are independent.

On the other hand, at N$^3$LO, the contact terms contain the same structures of nominal order $\mathcal{O}(p^4)$ for these partial waves. The only difference is that at N$^3$LO, the coefficients for these terms are composed of the N$^3$LO LECs ($O_{18,\ldots,40}$) [1]. The relevant terms of order $\mathcal{O}(p^4)$ for $^3P_2$ and $^3P_2$-$^3F_2$ at N$^3$LO read

$$
\begin{aligned}
V_{3P2}^{N^3LO} &= D_1 \frac{\pi p p' (\Delta_p + \Delta_{p'})}{\mathrm{m}^3}, \\
V_{3P2-3F2}^{N^3LO} &= D_2 \frac{\pi p p'^3}{\mathrm{m}^3 N_{p'}},
\end{aligned} \tag{1}
$$

in which $\Delta_p, \Delta_{p'}, N_{p'}$ are defined in Eq. (11). The $D_1$ and $D_2$ are

$$
\begin{aligned}
D_1 &= (-2O_{18} - O_{19} - O_{20} - 10O_{21} - 9O_{22} - 10O_{24} \\
&\quad - 10O_{25} + 10O_{26} - 20O_{27} - 2O_{28} - O_{29} - O_{30} \\
&\quad - 10O_{31} - 9O_{32} - 10O_{33} - 12O_{34} + 12O_{35} - 16O_{36} \\
&\quad - 10O_{37} - 14O_{38} + 14O_{39} - 12O_{40})/30, \\
D_2 &= -5\sqrt{\frac{3}{2}}(2O_{18} + O_{19} + O_{20} - O_{22} + 2O_{28} \\
&\quad + O_{29} + O_{30} - O_{32} + 2O_{34} - 2O_{35} - 4O_{36} + 4O_{38} \\
&\quad - 4O_{39} - 8O_{40}).
\end{aligned} \tag{2}
$$

In the present work, we promote these two additional terms of Eq. (1) from N$^3$LO to $V_{3P2}^{NLO}$ and $V_{3P2-3F2}^{NLO}$ in Eq. (22). This is equivalent to performing the following replacements,

$$
C_2^{3P2} \to C_2^{3P2} + D_1, \qquad C_1^{3PF2} \to C_1^{3PF2} + D_2. \tag{3}
$$

This way, we break the correlation between $C_2^{3P2}$, $C_1^{3PF2}$, and the other six combinations. We have now five independent

TABLE I. $\tilde{\chi}^2 = \sum_i (\delta^i - \delta^i_{\rm PWA93})^2$ of different chiral forces of partial waves up to $J \leq 2$.

| | Total | $^1S_0$ | $^3P_0$ | $^1P_1$ | $^3P_1$ | $^3S_1$ | $^3D_1$ | $\epsilon_1$ | $^1D_2$ | $^3D_2$ | $^3P_2$ | $^3F_2$ | $\epsilon_2$ |
|---|---|---|---|---|---|---|---|---|---|---|---|---|---|
| NNLO | 51.64 | 0.29 | 0.29 | 1.13 | 1.50 | 3.40 | 0.01 | 0.15 | 0.01 | 9.71 | 34.73 | 0.41 | 0.03 |
| NR-NNLO | 289.59 | 2.68 | 27.49 | 2.32 | 20.96 | 0.62 | 0.25 | 1.55 | 0.06 | 12.47 | 217.42 | 2.52 | 1.26 |
| NR-N$^3$LO-Idaho | 8.84 | 1.53 | 0.30 | 2.41 | 0.04 | 2.33 | 1.00 | 0.02 | 0.57 | 0.42 | 0.17 | 0.03 | 0.02 |
| NR-N$^3$LO-EKM | 16.08 | 13.45 | 0.29 | 0.34 | 0.06 | 0.01 | 0.13 | 0.01 | 0.02 | 0.43 | 0.12 | 1.22 | 0.00 |

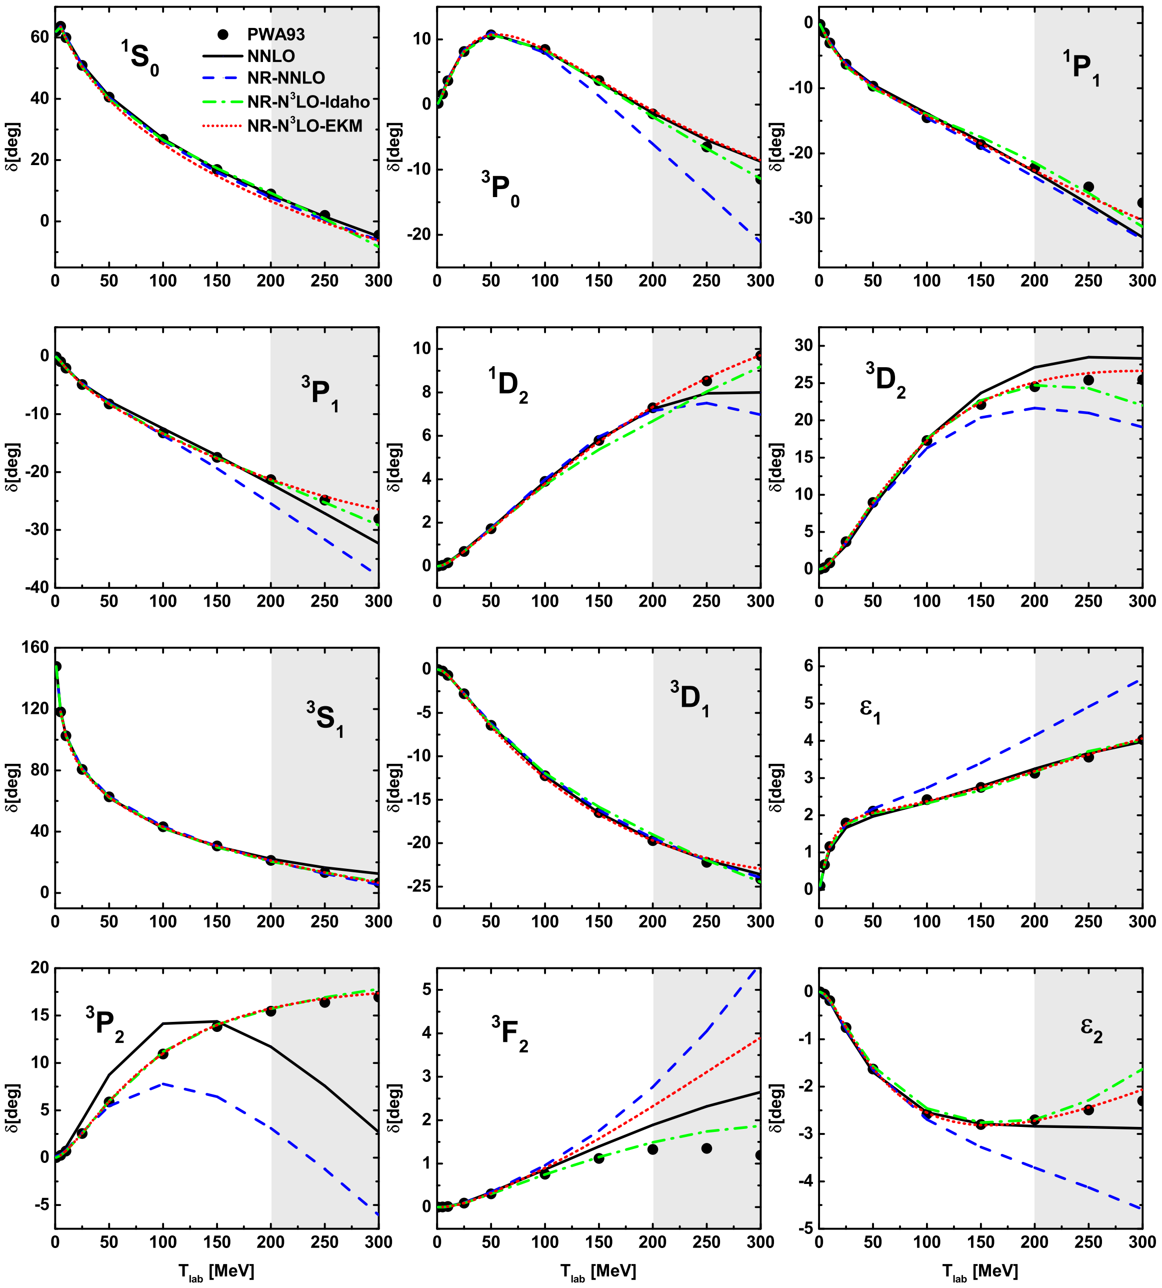


FIG. 1. $NN$ phase shifts for the partial waves with total angular momentum $J \leq 2$. The black solid lines denote the relativistic NNLO results obtained with a cutoff $\Lambda = 0.9$ GeV. For comparison, we also show the non-relativistic results up to NNLO (NR-NNLO, $\Lambda = 0.875$ GeV, blue dashed lines [2]) and N$^3$LO (NR-N$^3$LO-Idaho, $\Lambda = 0.5$ GeV, green dash-dotted lines [3, 4], and NR-N$^3$LO-EKM, $\Lambda = 0.9$ fm, red dotted lines [5, 6]). The black dots denote the empirical PWA93 phase shifts [12]. The shadows represent the energy regions not taken into account in the fitting.

combinations of LECs for the $J = 2$ partial waves instead of three. We have checked that the two combinations $D_1$ and $D_2$ only contribute to the ${}^3P_2$ and ${}^3P_2$-${}^3F_2$ partial waves, which leads to a much better description of the ${}^3P_2$ partial wave. Therefore, in total, we have 19 LECs for the NNLO potential presented in the main text.

## INFLUENCE OF CUTOFF VARIATIONS FROM 0.8 GEV TO 0.9 GEV

In Fig. 2, we compare the relativistic NNLO fits obtained with a cutoff of 0.9 GeV and 19 LECs and those obtained with a smaller cutoff of 0.8 GeV. With the cutoff switched to 0.8 GeV, we obtain a relatively better description of ${}^3P_0$, ${}^3D_2$, and ${}^3F_2$ for $T_{\rm lab} \leq 200$ MeV and thus a much smaller $\tilde{\chi}^2 \sim 5.3$. Clearly, the cutoff dependence is visible only for the ${}^3F_2$, ${}^3D_2$ phase shifts and the mixing angle $\epsilon_2$ at higher kinetic energies. This indicates that for these partial waves, inclusion of higher chiral order contributions is necessary.

For the ${}^3D_3$ partial wave to which no contact term contributes, the phase shifts are more sensitive to the choice of the cutoff as is shown in Fig. 6. This is the main reason why we stick to the cutoff of 0.9 GeV. However, we find that once the N$^3$LO contact terms are introduced, the cutoff dependence can be largely suppressed.

## COMPARISON WITH THE BONN POTENTIAL

For years, in relativistic studies of nuclear structure and reactions, the Bonn potential developed in the 1980's has been the only choice [14]. In Figs. 3 and 4, we compare the phase shifts for partial wave with $J \leq 7$. It is clear that on average the relativistic chiral nuclear force provides a better description of the PWA93 phase shifts than the Bonn potential, for example, ${}^1S_0$, ${}^3P_0$, ${}^3D_1$, and ${}^3D_3$.

## FIT TO THE GRANADA PWA

In the main text, we have fitted our relativistic chiral nuclear force to the Nijgemen 93 partial wave phase shifts [12], which have been used as benchmark purposes for most previous studies. Starting from 2013 [15], the Granada group has started a new partial wave analysis of the nucleon-nucleon scattering data, employing chiral TPE potentials, providing uncertainties, as well as taking into account correlations [16–18]. As a result, it is interesting to fit our relativistic chiral nuclear force to the Granada phaseshifts [17]. As uncertainties are provided in Ref. [17], we perform a standard $\chi^2$ fit. The results are shown in Fig. 5 labeled as "NNLO-G", in comparison with the results obtained by fitting to the Nijmegen phase shifts and the N$^3$LO results of Refs. [3–6]. Clearly, we can also obtain satisfactory fits. Comparing the Nijmegen and Granada phaseshifts, one can see some visable differences in certain channels, such as ${}^3P_2$, ${}^3F_2$, and $\varepsilon_2$, which is mainly due to the fact that charge symmetry breaking is considered for certain $P$-waves in Ref. [17]. One can see that the two N$^3$LO non-relativistic chrial nuclear forces yield results in better agreement with the Nijmegen PWA results. On the other hand, in the covariant framework, taking into account theoretical uncertainties, the two fits (to either the Nijmegen or the Granada phase shifts) are consistent with each other.

## COMPARISON WITH THE NONRELATIVISTIC N$^3$LO RESULTS FOR HIGHER PARTIAL WAVES

In Fig. 6, we compare the NR-N$^3$LO-Idaho [3, 4] and the NR-N$^3$LO-EKM [5, 6] chiral force with the relativistic NNLO chiral force for peripheral partial waves with $J \leq 4$ and $L \leq 4$. Higher partial waves are not explicitly shown since for them the OPE plays the dominant role.

The $\tilde{\chi}^2$ for each partial wave are collected in Table II. Clearly for these partial waves, the relativistic NNLO results are as good as or even slightly better than the nonrelativistic N$^3$LO results for $T_{\rm lab} \leq 200$ MeV except for ${}^3F_4$. For ${}^3D_3$ and ${}^1F_3$, our relativistic NNLO results and NR-N$^3$LO-EKM are not able to describe well the high-momentum data, while the NR-N$^3$LO-Idaho results miss the data for $T_{\rm lab} \in$ [100,200] MeV. For ${}^3F_3$, no results can reproduce the behavior above $T_{\rm lab} = 200$ MeV but the NR-N$^3$LO-Idaho results are slightly better. The large part of the $\tilde{\chi}^2$ for our relativistic NNLO results comes from ${}^3F_4$, in which the subleading TPE is strong such that it shifts the results well above the PWA93 phase shifts, while the NR-N$^3$LO-Idaho results behave much better. For the $G$-waves and the mixing angle $\epsilon_3$, all three results are in pretty good agreement with the empirical data below $T_{\rm lab} = 200$ MeV, while the NR-N$^3$LO-Idaho results tend to yield smaller values at higher energies.

Note for the peripheral partial waves shown in Fig. 6, visable differences between the Nijmegen results and the Granada results are found in the ${}^3D_3$, ${}^1F_3$, ${}^3F_3$, and ${}^3G_4$ channels. For these partial waves, the chiral phase shifts are predictions. Although the central values of the chiral nuclear forces agree better with the Nijmegen results, considering theoretical uncertainties, they should be viewed more or less equivalent, particularly for laboratory energies smaller than 200 MeV.

## THE BAYESIAN MODEL FOR UNCERTAINTY QUANTIFICATION

In this section, we briefly introduce the Bayesian model proposed first in Refs. [19–21] and further improved in Refs. [22–24].

In this approach, one first rewrites an observable $X$ in terms of dimensionless expansion coefficients $c_i$ as

$$X = X_{\rm ref}(c_0 + c_2 Q^2 + c_3 Q^3 + \cdots). \quad (4)$$

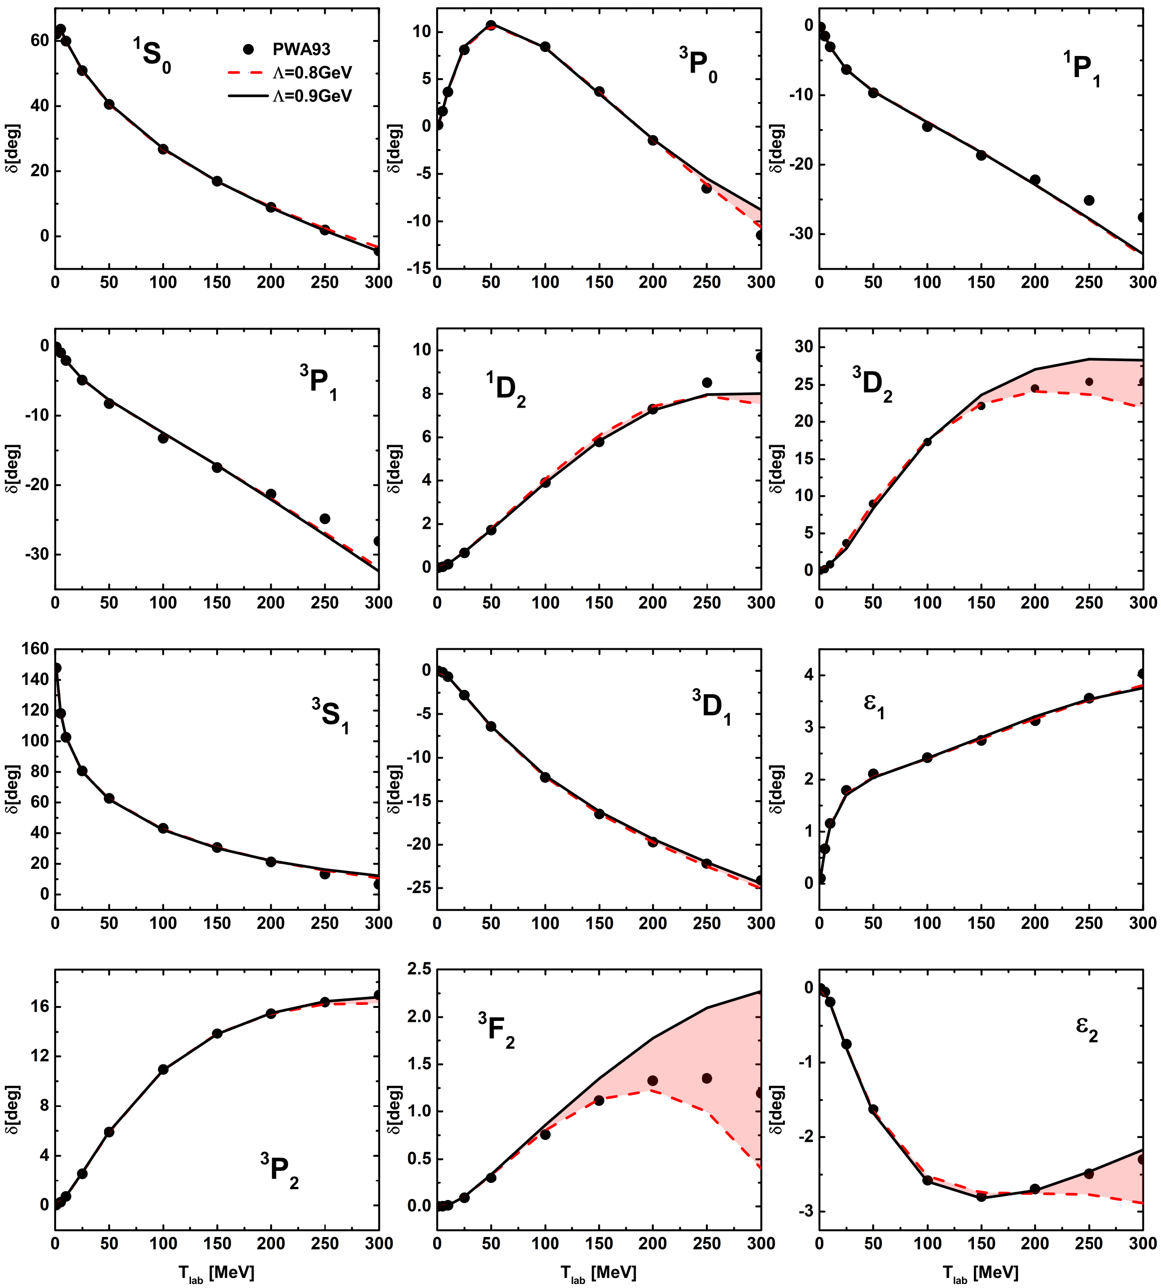


FIG. 2. $NN$ phase shifts for all the partial waves with $J \leq 2$ obtained with a variation of the cutoff from 0.8 GeV to 0.9 GeV. The relativistic NNLO results obtained with a cutoff of $\Lambda = 0.8$ GeV and $\Lambda = 0.9$ GeV are represented with red dashed lines and solid black lines, respectively. The uncertainties due to the cutoff variation are denoted by red shadows.

TABLE II. $\tilde{\chi}^2 = \sum_i (\delta^i - \delta^i_{\rm PWA93})^2$ of different chiral forces for partial waves shown in Fig. 6.

| | Total | $^3D_3$ | $^1F_3$ | $^3F_3$ | $^3F_4$ | $^3G_3$ | $\epsilon_3$ | $^1G_4$ | $^3G_4$ |
|---|---|---|---|---|---|---|---|---|---|
| NNLO | 0.98 | 0.03 | 0.03 | 0.21 | 0.70 | 0.00 | 0.01 | 0.00 | 0.00 |
| NR-N$^3$LO-Idaho | 1.73 | 0.58 | 0.73 | 0.13 | 0.12 | 0.00 | 0.01 | 0.01 | 0.15 |
| NR-N$^3$LO-EKM | 3.00 | 0.56 | 1.44 | 0.28 | 0.54 | 0.01 | 0.01 | 0.03 | 0.13 |

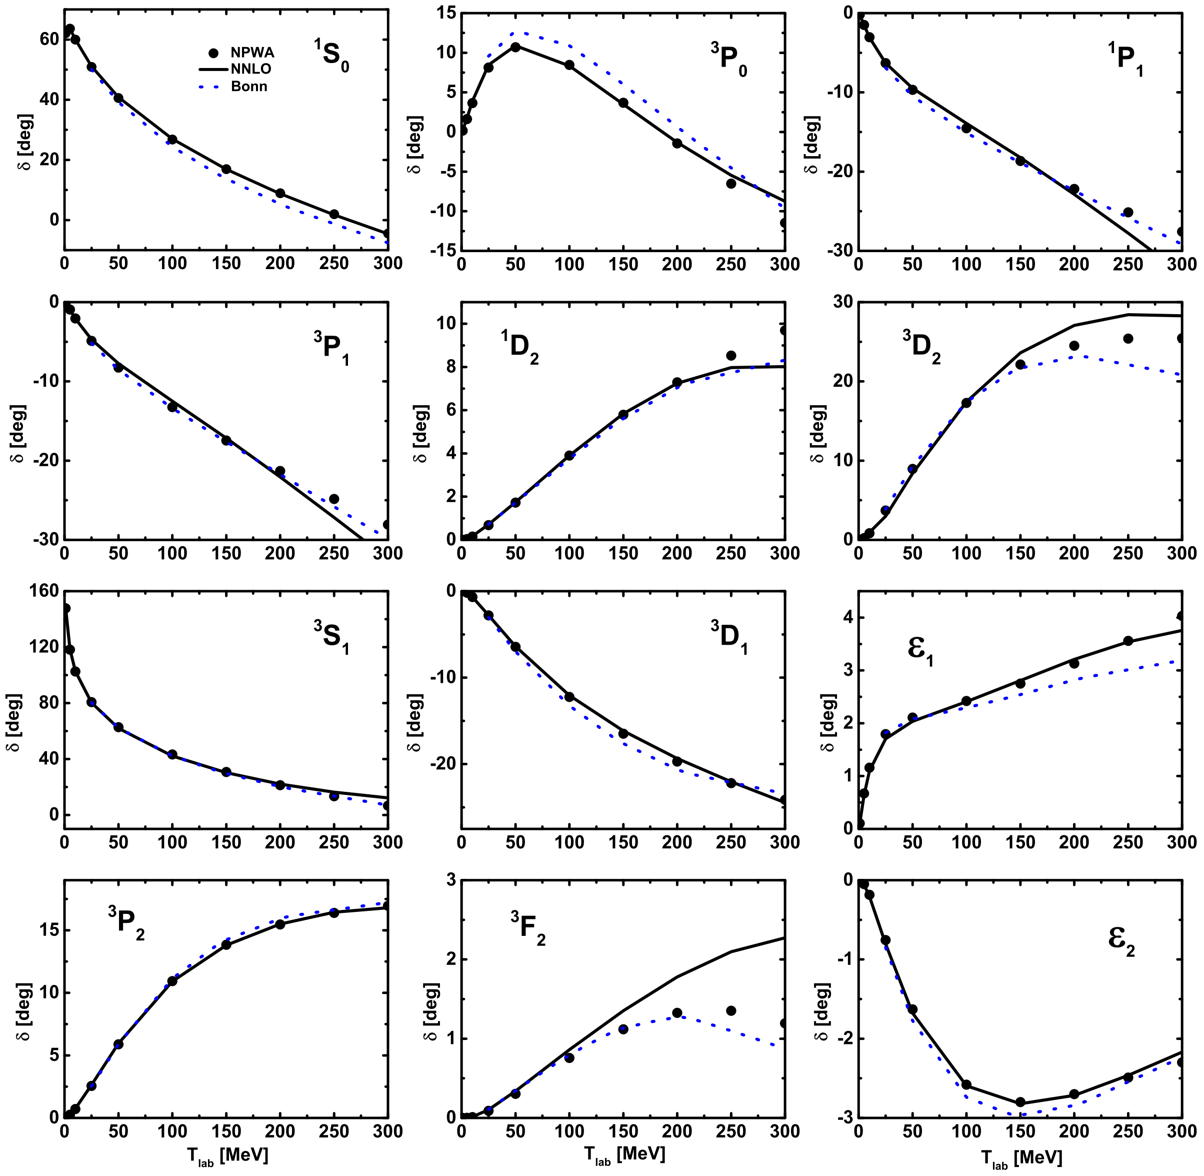


FIG. 3. $NN$ phase shifts for all the partial waves with $J \leq 2$ given by the relativistic NNLO chiral potential and the Bonn potential [13].

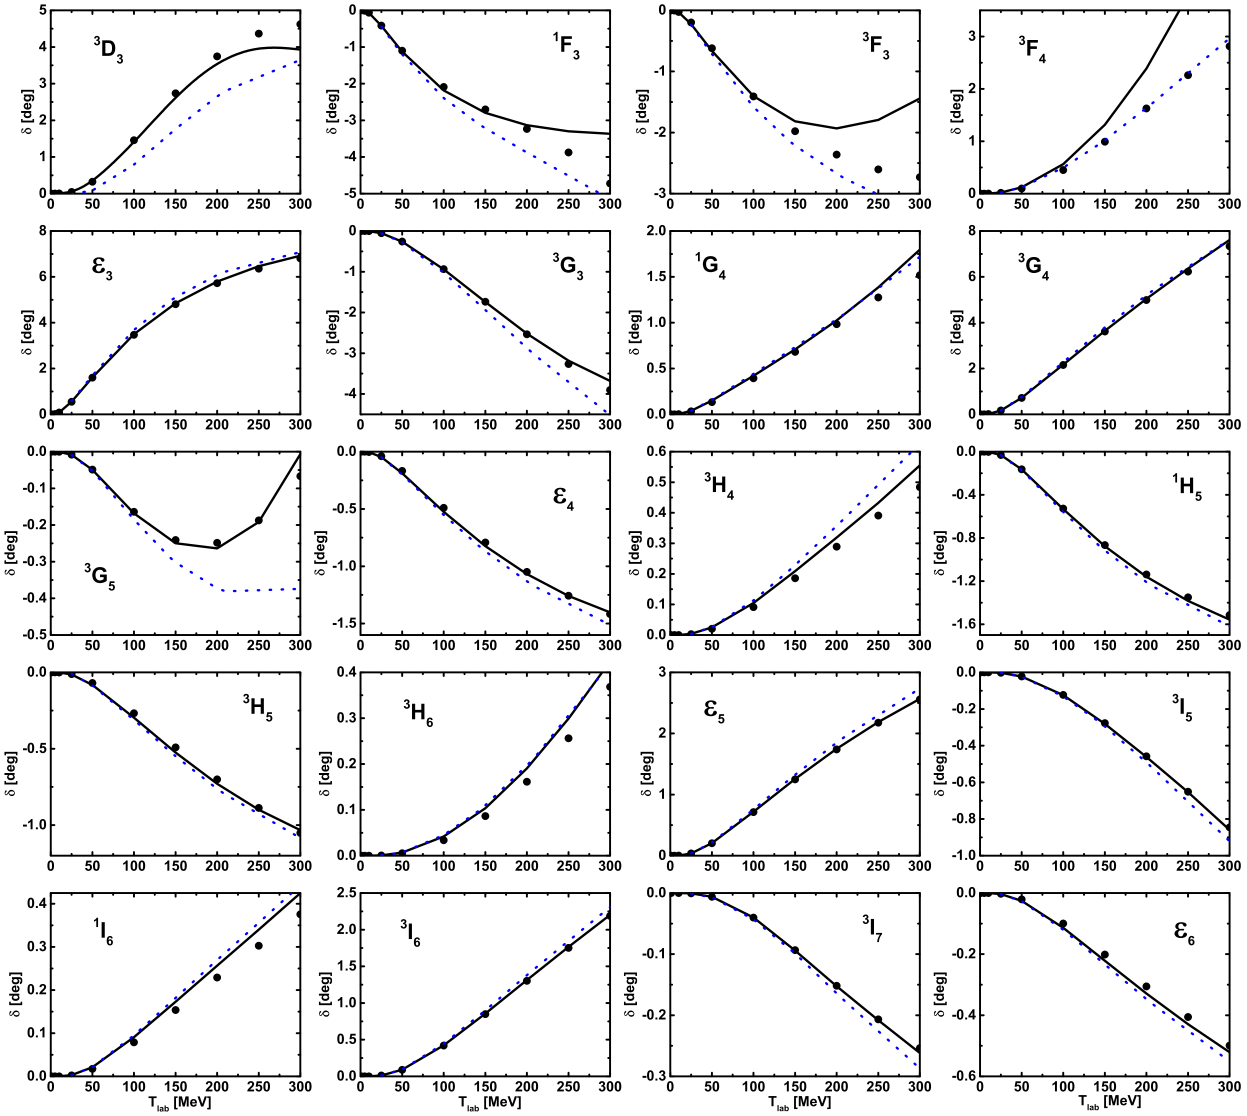


FIG. 4. $NN$ phase shifts for all the partial waves with $3 \leq J \leq 7$ given by the relativistic NNLO chiral potential and the Bonn potential [13].

The chiral expansion parameter $Q$ reads

$$Q = \mathrm{Max}\{\frac{p}{\Lambda_b}, \frac{m_\pi}{\Lambda_b}\}, \tag{5}$$

where $p$ is the nucleon momentum in the c.m. frame and $\Lambda_b$ is the cutoff. As is shown in the main text, since the optimum cutoff is determined to be 0.6 GeV at NLO but 0.9 GeV at NNLO, we adopt $\Lambda_b = 0.6$ GeV, which results in more conservative estimates of truncation uncertainties.

More specifically, at NNLO, it is suggested [22] that $X_{\mathrm{ref}}$ can be defined as

$$X_{\mathrm{ref}} = \mathrm{Max}\{|X^{\mathrm{LO}}|, \frac{|X^{\mathrm{LO}} - X^{\mathrm{NLO}}|}{Q^2}, \frac{|X^{\mathrm{NLO}} - X^{\mathrm{NNLO}}|}{Q^3}\}, \tag{6}$$

where $c_m = 1, m \in \{0, 2, 3\}$ instead of $X_{\mathrm{ref}} = |X^{\mathrm{LO}}|$ in order to avoid possible underestimation of $X_{\mathrm{ref}}$.

With the assumption that the next $h$ chiral orders dominate the truncation errors and given the knowledge of $\{c_{i\leq k}\}$, the dimensionless residue $\Delta_k \equiv \sum_{n=k+1}^{\infty} c_n Q^n \simeq \sum_{n=k+1}^{k+h} c_n Q^n$ obeys the following probability distribution

$$\mathrm{pr}_h(\Delta|c_{i\leq k}) = \frac{\int_0^\infty d\bar{c}\, \mathrm{pr}_h(\Delta|\bar{c})\mathrm{pr}(\bar{c}) \prod_{i\in A} \mathrm{pr}(c_i|\bar{c})}{\int_0^\infty d\bar{c}\, \mathrm{pr}(\bar{c}) \prod_{i\in A} \mathrm{pr}(c_i|\bar{c})}, \tag{7}$$

with $A = \{n \in \mathbf{N}_0 | n \leq k \wedge n \neq 1 \wedge n \neq m\}$ and

$$\mathrm{pr}_h(\Delta|\bar{c}) = [\prod_{i=k+1}^{k+h} \int_{-\infty}^{\infty} dc_i\, \mathrm{pr}(c_i|\bar{c})]\delta(\Delta - \sum_{j=k+1}^{k+h} c_j Q^j), \tag{8}$$

where $\bar{c}$ is the hyperparameter for the probability distribution function $\mathrm{pr}(c_i|\bar{c})$, which itself follows the log-uniform proba-

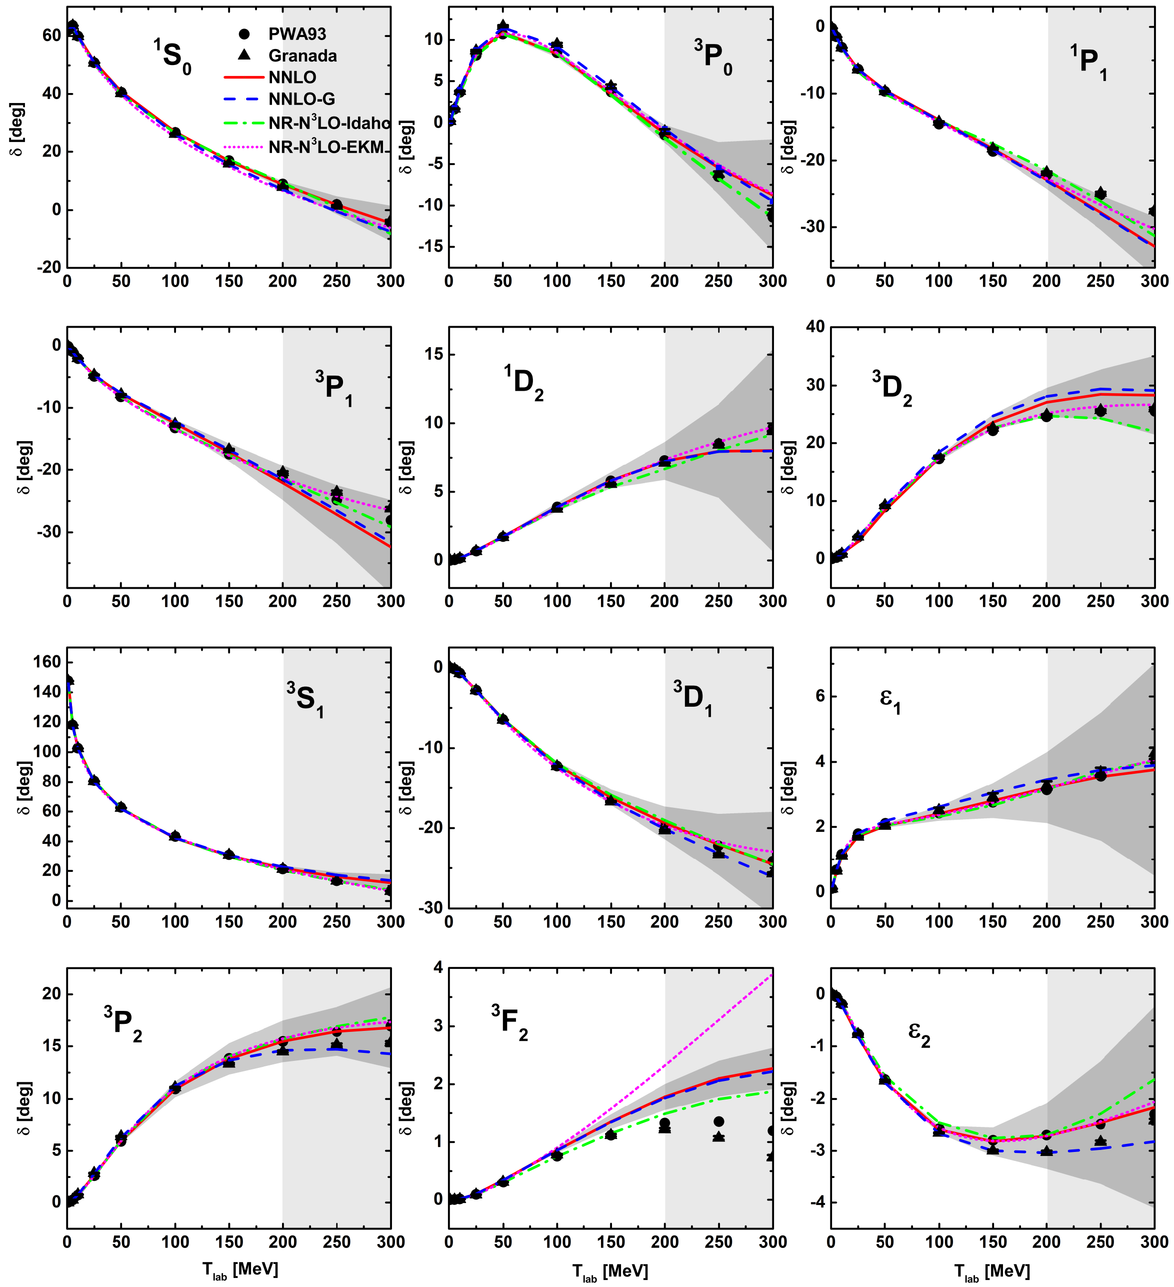


FIG. 5. $NN$ phase shifts for the partial waves with total angular momentum $J \le 2$. The red solid lines and the gray bands denote the relativistic NNLO results fitting to the empirical PWA93 phase shifts [12] obtained with a cutoff $\Lambda = 0.9$ GeV and 68% DoB truncation errors. The results fitting to the Granada data [17] are depicted with blue dashed lines labeled as "NNLO-G". For comparison, we also show the non-relativistic results up to N$^3$LO (NR-N$^3$LO-Idaho, $\Lambda = 0.5$ GeV, green dash-dotted lines [3, 4], and NR-N$^3$LO-EKM, $\Lambda = 0.9$ fm, magenta dotted lines [5, 6]). The black solid circles and triangles denote the empirical PWA93 phase shifts [12] and those of the Granada Group [17]. The shadows represent the energy regions not taken into account in the fitting.

bility distribution as

$$\mathrm{pr}(\bar{c}) = \frac{1}{\ln(\bar{c}_>/\bar{c}_<)} \frac{1}{\bar{c}} \theta(\bar{c} - \bar{c}_<)\theta(\bar{c}_> - \bar{c}). \qquad (9)$$

Following Refs. [20, 22], we utilize the Gaussian prior for $\mathrm{pr}(c_i|\bar{c})$ as

$$\mathrm{pr}(c_i|\bar{c}) = \frac{1}{\sqrt{2\pi}\bar{c}}\, e^{-c_i^2/2\bar{c}^2}. \qquad (10)$$

In the practical application, as is suggested in Ref. [20], it is efficient to take $h = 10$, $\bar{c}_< = 0.5$ and $\bar{c}_> = 10.0$. For

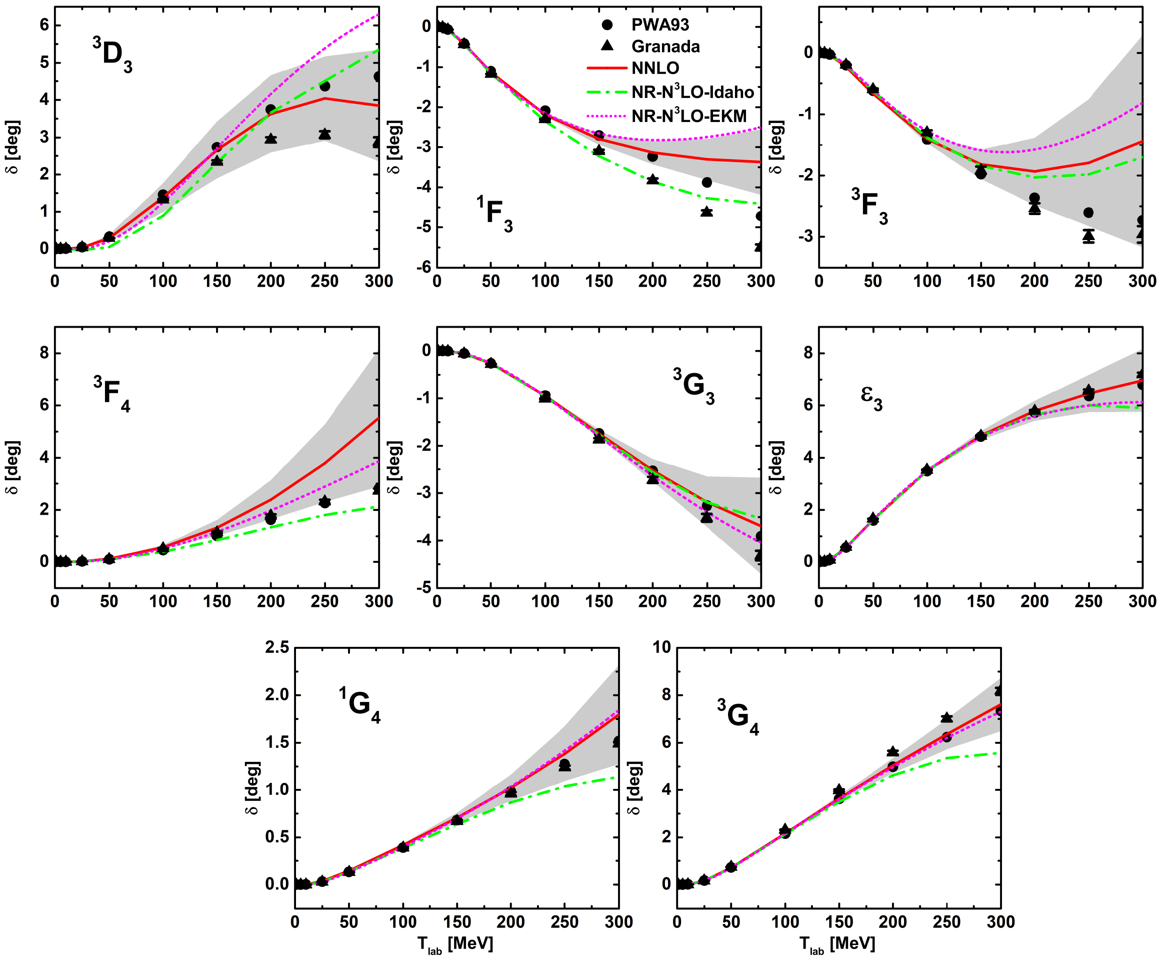


FIG. 6. Same as Fig. 5 but for peripheral partial waves with $J \leq 4$ and $L \leq 4$. Note that for these partial waves, the chiral results are predictions and independent from the partial wave analyses.

any given degree-of-belief (DoB) interval, the truncation uncertainties $\Delta X = X_{\rm ref}\Delta_k$ can be numerically obtained by integrating over $\Delta$.

## CONTACT TERMS

In this section, we explicitly present the partial wave contributions of the LO and NLO contact terms of our relativistic chiral nuclear force. For simplification, we define

$$\Delta_p = E_p - m, \qquad \Delta_{p'} = E_{p'} - m, \tag{11}$$
$$N_p = E_p + m, \qquad N_{p'} = E_{p'} + m, \tag{12}$$
$$\Sigma = E_p E_{p'} + m^2, \qquad \Gamma = E_p E_{p'} - m^2. \tag{13}$$

The contributions of contact terms to each partial wave then read

$$\begin{aligned}
V_{1S0}^{LO} &= 2\pi\left(2C_1^{1S0} + C_2^{1S0}\frac{\Gamma}{\mathrm{m}^2}\right)\\
V_{3P0}^{LO} &= -\frac{2\pi C^{3P0}pp'}{\mathrm{m}^2}\\
V_{1P1}^{LO} &= -\frac{2\pi C^{1P1}pp'}{3\mathrm{m}^2}\\
V_{3P1}^{LO} &= -\frac{4\pi C^{3P1}pp'}{3\mathrm{m}^2}\\
V_{3S1}^{LO} &= C_1^{3S1}\frac{4\pi\left(7\mathrm{m}^2 + 2\mathrm{m}(E_p + E_{p'}) - 2E_pE_{p'}\right)}{9\mathrm{m}^2}\\
&\quad + C_2^{3S1}\frac{2}{3}\pi\frac{\Gamma}{\mathrm{m}^2}\\
V_{3D1}^{LO} &= C^{3D1}\frac{8\pi\Delta_p\Delta_{p'}}{9\mathrm{m}^2}\\
V_{3SD1}^{LO} &= \frac{2\sqrt{2}\pi\Delta_{p'}(6\mathrm{m}C_1^{3SD1} + C_2^{3SD1}\Delta_p)}{9\mathrm{m}^2}
\end{aligned} \tag{14}$$

$$
\begin{aligned}
V_{1S0}^{NLO} &= C_1^{1S0} + C_2^{1S0}\frac{(\Delta_p + \Delta_{p'})}{\mathrm{m}} \\
&+ C_3^{1S0}\frac{\left(p^2\Delta_p E_{p'} + p'^2\Delta_{p'}E_p\right)}{\mathrm{m}^4} \\
&+ C_4^{1S0}\frac{p^2p'^2}{\mathrm{m}^2N_pN_{p'}} + C_5^{1S0}\frac{\Sigma\sqrt{s}(\Delta_p + \Delta_{p'})}{\mathrm{m}^4} \\
&+ C_6^{1S0}\frac{\sqrt{s}\Delta_p\Delta_{p'}}{\mathrm{m}^3} + C_7^{1S0}\frac{(s + \Delta_pE_p + \Delta_{p'}E_{p'})}{\mathrm{m}^2} \\
&+ C_8^{1S0}\frac{\Gamma s}{\mathrm{m}^4} + C_9^{1S0}\frac{(\Delta_pE_p + \Delta_{p'}E_{p'})}{\mathrm{m}^2} \\
&+ C_{10}^{1S0}\frac{\Delta_p\Delta_{p'}(E_p + E_{p'})}{\mathrm{m}^3} + C_{11}^{1S0}\frac{\Delta_p\Delta_{p'}E_pE_{p'}}{\mathrm{m}^4}
\end{aligned} \tag{15}
$$

$$
\begin{aligned}
V_{3P0}^{NLO} &= C_1^{3P0}\frac{pp'}{\mathrm{m}^2} + C_2^{3P0}\frac{pp'(\Delta_p + \Delta_{p'})}{\mathrm{m}^3} \\
&+ C_3^{3P0}\frac{p^3p'^3}{\mathrm{m}^4N_pN_{p'}} + C_4^{3P0}\frac{pp'\sqrt{s}}{\mathrm{m}^3} \\
&+ C_5^{3P0}\frac{pp'\sqrt{s}(\Delta_p + \Delta_{p'})}{\mathrm{m}^4} + C_6^{3P0}\frac{pp's}{\mathrm{m}^4} \\
&+ C_7^{3P0}\frac{pp'(\Delta_pE_p + \Delta_{p'}E_{p'})}{\mathrm{m}^4}
\end{aligned} \tag{16}
$$

$$
\begin{aligned}
V_{1P1}^{NLO} &= C_1^{1P1}\frac{pp'}{\mathrm{m}^2} + C_2^{1P1}\frac{pp'(\Delta_p + \Delta_{p'})}{\mathrm{m}^3} \\
&+ C_3^{1P1}\frac{p^3p'^3}{\mathrm{m}^4N_pN_{p'}} + C_4^{1P1}\frac{pp'\sqrt{s}(E_p + E_{p'})}{\mathrm{m}^4} \\
&+ C_5^{1P1}\frac{pp's}{\mathrm{m}^4} + C_6^{1P1}\frac{pp'(\Delta_pE_p + \Delta_{p'}E_{p'})}{\mathrm{m}^4}
\end{aligned} \tag{17}
$$

$$
\begin{aligned}
V_{3P1}^{NLO} &= C_1^{3P1}\frac{pp'}{\mathrm{m}^2} + C_2^{3P1}\frac{pp'(\Delta_p + \Delta_{p'})}{\mathrm{m}^3} \\
&+ C_3^{3P1}\frac{p^3p'^3}{\mathrm{m}^4N_pN_{p'}} + C_4^{3P1}\frac{pp'\sqrt{s}(E_p + E_{p'})}{\mathrm{m}^4} \\
&+ C_5^{3P1}\frac{pp's}{\mathrm{m}^4} + C_6^{3P1}\frac{pp'(\Delta_pE_p + \Delta_{p'}E_{p'})}{\mathrm{m}^4}
\end{aligned} \tag{18}
$$

$$
\begin{aligned}
V_{3S1}^{NLO} &= C_1^{3S1}\frac{\Delta_p + \Delta_{p'}}{\mathrm{m}} + C_2^{3S1}\frac{p^2\Delta_p + p'^2\Delta_{p'}}{\mathrm{m}^3} \\
&+ C_3^{3S1}\frac{p^2p'^2}{\mathrm{m}^2N_pN_{p'}} + C_4^{3S1}\frac{\Delta_p\Delta_{p'}\left(p^2 + p'^2\right)}{\mathrm{m}^4} \\
&+ C_5^{3S1}\frac{\sqrt{s}\left(p^2 + p'^2\right)}{\mathrm{m}^3} + C_6^{3S1}\frac{\sqrt{s}\Delta_p\Delta_{p'}}{\mathrm{m}^3} \\
&+ C_7^{3S1}\frac{-4\mathrm{m}^2 + s + \Delta_pE_p + \Delta_{p'}E_{p'}}{\mathrm{m}^2} \\
&+ C_8^{3S1}\frac{s(\Delta_p + \Delta_{p'})}{\mathrm{m}^3} + C_9^{3S1}\frac{s\Delta_p\Delta_{p'}}{\mathrm{m}^4} \\
&+ C_{10}^{3S1}\frac{\Delta_pE_p + \Delta_{p'}E_{p'}}{\mathrm{m}^2} + C_{11}^{3S1}\frac{\Delta_p\Delta_{p'}(E_p + E_{p'})}{\mathrm{m}^3} \\
&+ C_{12}^{3S1}\frac{\sqrt{s}\Delta_p\Delta_{p'}(E_p + E_{p'})}{\mathrm{m}^4} + C_{13}^{3S1}\frac{\Delta_p\Delta_{p'}E_pE_{p'}}{\mathrm{m}^4}
\end{aligned} \tag{19}
$$

$$
\begin{aligned}
V_{3D1}^{NLO} &= C_1^{3D1}\frac{\Delta_p\Delta_{p'}}{\mathrm{m}^2} + C_2^{3D1}\frac{\Delta_p\Delta_{p'}\left(p^2 + p'^2\right)}{\mathrm{m}^4} \\
&+ C_3^{3D1}\frac{\sqrt{s}\left(p^2\Delta_{p'} + p'^2\Delta_p\right)}{2\mathrm{m}^4} + C_4^{3D1}\frac{p^2p'^2s}{\mathrm{m}^4N_pN_{p'}} \\
&+ C_5^{3D1}\frac{\Delta_p\Delta_{p'}(E_p + E_{p'})}{\mathrm{m}^3} + C_6^{3D1}\frac{\Delta_p\Delta_{p'}E_pE_{p'}}{\mathrm{m}^4}
\end{aligned} \tag{20}
$$

$$
\begin{aligned}
V_{3SD1}^{NLO} &= C_1^{3SD1}\frac{\sqrt{2}\Delta_{p'}}{9\mathrm{m}} + C_2^{3SD1}\frac{\sqrt{2}\Delta_{p'}{}^2N_{p'}}{9\mathrm{m}^3} \\
&+ C_3^{3SD1}\frac{\sqrt{2}\Delta_p\Delta_{p'}}{9\mathrm{m}^2} + C_4^{3SD1}\frac{\sqrt{2}\Delta_p\Delta_{p'}\left(p^2 + p'^2\right)}{9\mathrm{m}^4} \\
&+ C_5^{3SD1}\frac{\sqrt{2s}\Delta_{p'}\left(\sqrt{s} + N_{p'}\right)}{9\mathrm{m}^3} \\
&+ C_6^{3SD1}\frac{\sqrt{2s}\Delta_p\Delta_{p'}}{9\mathrm{m}^3} + C_7^{3SD1}\frac{\sqrt{2}s\Delta_{p'}}{9\mathrm{m}^3} \\
&+ C_8^{3SD1}\frac{\sqrt{2}s\Delta_p\Delta_{p'}}{9\mathrm{m}^4} + C_9^{3SD1}\frac{\sqrt{2}\Delta_{p'}E_{p'}}{9\mathrm{m}^2} \\
&+ C_{10}^{3SD1}\frac{\sqrt{2}\Delta_p\Delta_{p'}E_{p'}}{9\mathrm{m}^3} + C_{11}^{3SD1}\frac{\sqrt{2s}\Delta_p\Delta_{p'}(E_p + E_{p'})}{9\mathrm{m}^4} \\
&+ C_{12}^{3SD1}\frac{\sqrt{2}\Delta_p\Delta_{p'}E_p}{9\mathrm{m}^3} \\
&+ C_{13}^{3SD1}\frac{\sqrt{2}\Delta_p\Delta_{p'}E_pE_{p'}}{9\mathrm{m}^4}
\end{aligned} \tag{21}
$$

$$
\begin{aligned}
V_{1D2}^{NLO} &= \frac{C^{1D2}p^2p'^2}{\mathrm{m}^4} \\
V_{3D2}^{NLO} &= \frac{C^{3D2}p^2p^2}{\mathrm{m}^4} \\
V_{3P2}^{NLO} &= C_1^{3P2}\frac{pp'}{\mathrm{m}^2} + C_2^{3P2}\frac{pp'(\Delta_p + \Delta_{p'})}{\mathrm{m}^3} \\
&+ C_3^{3P2}\frac{p^3p'^3}{\mathrm{m}^4N_pN_{p'}} \\
V_{3F2}^{NLO} &= C_3^{3F2}\frac{p^3p'^3}{\mathrm{m}^4N_pN_{p'}} \\
V_{3P2-3F2}^{NLO} &= C_1^{3PF2}\frac{2\sqrt{\frac{2}{3}}}{25}\frac{pp'^3}{\mathrm{m}^3N_{p'}} \\
&+ C_2^{3PF2}\frac{\sqrt{\frac{2}{3}}p^3p'^3}{25\mathrm{m}^4N_pN_{p'}}
\end{aligned} \tag{22}
$$

Note that a factor of $\pi$ is omitted in Eqs. (15-22). The partial wave combinations in terms of the LECs appear in the covariant Lagrangians are given as follows.

$$
\begin{aligned}
C_1^{1S0} &= O_1 + O_2 + 3O_3 - 6O_4 \\
C_2^{1S0} &= O_1 + 4(O_2 + O_3 - 3O_4) \\
C^{3P0} &= O_1 - 4(O_2 + O_3 + 3O_4) \\
C^{1P1} &= O_1 + 4O_4 \\
C^{3P1} &= O_1 - 2O_2 + 2O_3 \\
C_1^{3S1} &= O_1 + O_2 - O_3 + 2O_4 \\
C_2^{3S1} &= 3O_1 + 4O_2 - 4O_3 - 4O_4 \\
C^{3D1} &= O_1 + O_2 - O_3 + 2O_4 \\
C_1^{3SD1} &= O_1 + O_2 - O_3 + 2O_4 \\
C_1^{3SD1} &= O_1 + 4O_2 - 4O_3 - 4O_4
\end{aligned} \tag{23}
$$

$$
\begin{aligned}
C_1^{1S0} &= -4O_{14} - 4O_{15} - 12O_{16} + 24O_{17} \\
C_2^{1S0} &= -O_{10} - O_{11} - 3O_{12} + 6O_{13} - O_{14} \\
&\quad - 7O_{15} - 5O_{16} + 18O_{17} + 2O_5 + O_6 - 2O_7 + 2O_9 \\
C_3^{1S0} &= -\frac{O_{10}}{2} - 2O_{11} - 2O_{12} + 6O_{13} + \frac{O_{14}}{2} + 2O_{15} \\
&\quad + 2O_{16} - 6O_{17} + \frac{O_6}{2} - \frac{3O_7}{2} + \frac{3O_9}{2} \\
C_4^{1S0} &= -\frac{4O_{10}}{3} - 4O_{11} - 4O_{12} + \frac{32O_{13}}{3} - \frac{4O_{14}}{3} - 4O_{15} \\
&\quad - 4O_{16} + \frac{32O_{17}}{3} + 2O_5 + 2O_6 - \frac{10O_7}{3} + \frac{4O_8}{3} + \frac{8O_9}{3} \\
C_5^{1S0} &= 2O_6 - 4O_7 + 2O_8 \\
C_6^{1S0} &= 4O_6 - 8O_7 + 4O_8 \\
C_7^{1S0} &= O_{14} + O_{15} + 3O_{16} - 6O_{17} \\
C_8^{1S0} &= \frac{O_{14}}{2} + 2O_{15} + 2O_{16} - 6O_{17} + 2O_6 - 6O_7 \\
C_9^{1S0} &= -O_{10} - O_{11} - 3O_{12} + 6O_{13} + O_6 - 2O_7 + 2O_9 \\
C_{10}^{1S0} &= -\frac{5O_{10}}{6} - 2O_{11} - 2O_{12} + \frac{14O_{13}}{3} + \frac{O_{14}}{6} + 2O_{15} \\
&\quad + 2O_{16} - \frac{22O_{17}}{3} + \frac{3O_6}{2} - \frac{11O_7}{6} + \frac{4O_8}{3} + \frac{7O_9}{6} \\
C_{11}^{1S0} &= -\frac{O_{10}}{3} - \frac{4O_{13}}{3} - \frac{O_{14}}{3} - \frac{4O_{17}}{3} + O_6 - \frac{O_7}{3} \\
&\quad + \frac{4O_8}{3} - \frac{O_9}{3}
\end{aligned} \tag{24}
$$

$$
\begin{aligned}
C_1^{3P0} &= \frac{2O_{10}}{3} + \frac{2O_{11}}{3} - \frac{2O_{12}}{3} + \frac{4O_{13}}{3} + \frac{8O_{14}}{3} - \frac{22O_{15}}{3} \\
&\quad - \frac{26O_{16}}{3} - \frac{68O_{17}}{3} - 2O_5 + 2O_6 + \frac{8O_7}{3} - \frac{8O_8}{3} + \frac{8O_9}{3} \\
C_2^{3P0} &= \frac{5O_{10}}{6} - 2O_{11} - 2O_{12} - \frac{14O_{13}}{3} - \frac{O_{14}}{6} + 2O_{15} \\
&\quad + 2O_{16} + \frac{22O_{17}}{3} + \frac{3O_6}{2} + \frac{11O_7}{6} - \frac{4O_8}{3} - \frac{7O_9}{6} \\
C_3^{3P0} &= \frac{O_{10}}{3} + \frac{4O_{13}}{3} + \frac{O_{14}}{3} + \frac{4O_{17}}{3} + O_6 + \frac{O_7}{3} \\
&\quad - \frac{4O_8}{3} + \frac{O_9}{3} \\
C_4^{3P0} &= 4O_6 + 8O_7 - 4O_8 \\
C_5^{3P0} &= 2O_6 + 4O_7 - 2O_8 \\
C_6^{3P0} &= -\frac{O_{14}}{2} + 2O_{15} + 2O_{16} + 6O_{17} + 2O_6 + 6O_7 \\
C_7^{3P0} &= \frac{O_{10}}{2} - 2O_{11} - 2O_{12} - 6O_{13} - \frac{O_{14}}{2} + 2O_{15} \\
&\quad + 2O_{16} + 6O_{17} + \frac{O_6}{2} + \frac{3O_7}{2} - \frac{3O_9}{2}
\end{aligned} \tag{25}
$$

$$
\begin{aligned}
C_1^{1P1} &= \frac{2O_{10}}{3} + \frac{2O_{11}}{3} + 2O_{12} - 4O_{13} + \frac{4O_{14}}{3} + \frac{2O_{15}}{3} \\
&\quad + 2O_{16} - \frac{4O_{17}}{3} - \frac{2O_5}{3} + \frac{2O_6}{3} - \frac{4O_7}{3} - \frac{4O_9}{3} \\
C_2^{1P1} &= \frac{O_{10}}{2} + \frac{4O_{11}}{3} + \frac{4O_{12}}{3} - \frac{10O_{13}}{3} + \frac{O_{14}}{6} + \frac{4O_{15}}{3} \\
&\quad + \frac{4O_{16}}{3} - \frac{14O_{17}}{3} + \frac{O_6}{2} - \frac{7O_7}{6} - \frac{5O_9}{6} \\
C_3^{1P1} &= \frac{O_{10}}{3} + \frac{4O_{11}}{3} + \frac{4O_{12}}{3} - 4O_{13} + \frac{O_{14}}{3} + \frac{4O_{15}}{3} \\
&\quad + \frac{4O_{16}}{3} - 4O_{17} + \frac{O_6}{3} - O_7 - O_9 \\
C_4^{1P1} &= \frac{2O_6}{3} - \frac{4O_7}{3} - \frac{2O_8}{3} \\
C_5^{1P1} &= -\frac{O_{14}}{6} - \frac{2O_{17}}{3} + \frac{2O_6}{3} - \frac{2O_7}{3} \\
C_6^{1P1} &= \frac{O_{10}}{6} + \frac{2O_{13}}{3} - \frac{O_{14}}{6} - \frac{2O_{17}}{3} + \frac{O_6}{6} - \frac{O_7}{6} + \frac{O_9}{6}
\end{aligned} \tag{26}
$$

$$
\begin{aligned}
C_1^{3P1} &= \frac{2O_{10}}{3} + \frac{2O_{11}}{3} - \frac{2O_{12}}{3} + \frac{4O_{13}}{3} + 2O_{14} - 2O_{15} \\
&+ 2O_{16} + \frac{4O_{17}}{3} + \frac{4O_5}{3} - \frac{4O_6}{3} - \frac{2O_7}{3} - \frac{4O_8}{3} - \frac{2O_9}{3} \\
C_2^{3P1} &= \frac{2O_{10}}{3} + \frac{4O_{15}}{3} - \frac{4O_{16}}{3} - O_6 - \frac{2O_7}{3} \\
&- \frac{2O_8}{3} - \frac{4O_9}{3} \\
C_3^{3P1} &= \frac{O_{10}}{3} + \frac{2O_{11}}{3} - \frac{2O_{12}}{3} + \frac{O_{14}}{3} + \frac{2O_{15}}{3} - \frac{2O_{16}}{3} \\
&- \frac{2O_6}{3} - O_7 - \frac{2O_8}{3} - O_9 \\
C_4^{3P1} &= -\frac{4O_6}{3} - \frac{4O_8}{3} \\
C_5^{3P1} &= -\frac{O_{14}}{3} + \frac{2O_{15}}{3} - \frac{2O_{16}}{3} - \frac{4O_6}{3} + \frac{4O_7}{3} \\
C_6^{3P1} &= \frac{O_{10}}{3} - \frac{2O_{11}}{3} + \frac{2O_{12}}{3} - \frac{O_{14}}{3} + \frac{2O_{15}}{3} - \frac{2O_{16}}{3} \\
&- \frac{O_6}{3} + \frac{O_7}{3} - \frac{O_9}{3}
\end{aligned} \tag{27}
$$

$$
\begin{aligned}
C_1^{3S1} &= -O_{10} - O_{11} + O_{12} - 2O_{13} - O_{14} - \frac{5O_{15}}{3} \\
&+ \frac{5O_{16}}{3} - \frac{2O_{17}}{3} - \frac{2O_5}{3} - \frac{O_6}{3} + \frac{2O_7}{3} - \frac{2O_9}{3} \\
C_2^{3S1} &= -\frac{O_{10}}{2} - \frac{2O_{11}}{3} + \frac{2O_{12}}{3} - \frac{2O_{13}}{3} + \frac{O_{14}}{2} + \frac{2O_{15}}{3} \\
&- \frac{2O_{16}}{3} + \frac{2O_{17}}{3} - \frac{O_6}{6} - \frac{O_7}{6} + \frac{O_9}{6} \\
C_3^{3S1} &= -\frac{4O_{10}}{3} - \frac{4O_{11}}{9} + \frac{4O_{12}}{3} - \frac{4O_{14}}{9} + \frac{4O_{15}}{9} + \frac{4O_{16}}{9} \\
&+ \frac{16O_{17}}{9} - \frac{2O_5}{3} - \frac{2O_6}{3} + \frac{14O_7}{9} + \frac{4O_8}{9} + \frac{4O_9}{9} \\
C_4^{3S1} &= -\frac{5O_{10}}{18} - \frac{4O_{11}}{9} + \frac{4O_{12}}{9} - \frac{2O_{13}}{9} + \frac{5O_{14}}{18} + \frac{4O_{15}}{9} \\
&- \frac{4O_{16}}{9} + \frac{2O_{17}}{9} - \frac{O_6}{6} - \frac{O_7}{6} + \frac{O_9}{6} \\
C_5^{3S1} &= -\frac{2O_6}{3} + \frac{4O_7}{3} + 2O_8 \\
C_6^{3S1} &= -\frac{4O_6}{3} + \frac{8O_7}{9} + \frac{20O_8}{9} \\
C_7^{3S1} &= O_{14} + O_{15} - O_{16} + 2O_{17} \\
C_8^{3S1} &= \frac{O_{14}}{2} + \frac{2O_{15}}{3} - \frac{2O_{16}}{3} + \frac{2O_{17}}{3} - \frac{2O_6}{3} - \frac{2O_7}{3} \\
C_9^{3S1} &= \frac{5O_{14}}{18} + \frac{4O_{15}}{9} - \frac{4O_{16}}{9} + \frac{2O_{17}}{9} - \frac{2O_6}{3} - \frac{2O_7}{3} \\
C_{10}^{3S1} &= -O_{10} - O_{11} + O_{12} - 2O_{13} - \frac{O_6}{3} + \frac{2O_7}{3} - \frac{2O_9}{3} \\
C_{11}^{3S1} &= -\frac{5O_{10}}{6} + \frac{2O_{11}}{9} + \frac{2O_{12}}{3} + \frac{2O_{13}}{3} + \frac{O_{14}}{6} + \frac{14O_{15}}{9} \\
&- \frac{2O_{16}}{3} + 2O_{17} - \frac{O_6}{2} + \frac{23O_7}{18} + \frac{4O_8}{9} + \frac{13O_9}{18} \\
C_{12}^{3S1} &= -\frac{2O_6}{3} + \frac{4O_7}{9} + \frac{10O_8}{9} \\
C_{13}^{3S1} &= -\frac{O_{10}}{3} + \frac{8O_{11}}{9} + \frac{4O_{13}}{3} - \frac{O_{14}}{3} + \frac{8O_{15}}{9} + \frac{4O_{17}}{3} \\
&- \frac{O_6}{3} + O_7 + \frac{4O_8}{9} + O_9
\end{aligned} \tag{28}
$$

$$C_1^{3D1} = -\frac{O_{10}}{3} + \frac{10O_{11}}{9} + \frac{2O_{12}}{3} + \frac{8O_{13}}{3} - \frac{11O_{14}}{9} + \frac{2O_{15}}{9} + \frac{14O_{16}}{9} + \frac{8O_{17}}{9} + \frac{O_7}{9} + \frac{2O_8}{9} + \frac{17O_9}{9}$$
$$C_2^{3D1} = -\frac{2O_{10}}{9} - \frac{2O_{11}}{9} + \frac{2O_{12}}{9} - \frac{4O_{13}}{9} + \frac{2O_{14}}{9} + \frac{2O_{15}}{9} - \frac{2O_{16}}{9} + \frac{4O_{17}}{9}$$
$$C_3^{3D1} = \frac{16O_7}{9} + \frac{16O_8}{9}$$
$$C_4^{3D1} = \frac{2O_{14}}{9} + \frac{2O_{15}}{9} - \frac{2O_{16}}{9} + \frac{4O_{17}}{9}$$
$$C_5^{3D1} = -\frac{O_{10}}{3} + \frac{10O_{11}}{9} + \frac{2O_{12}}{3} + \frac{8O_{13}}{3} - \frac{O_{14}}{3} + \frac{10O_{15}}{9} + \frac{2O_{16}}{3} + \frac{8O_{17}}{3} + \frac{5O_7}{9} + \frac{2O_8}{9} + \frac{13O_9}{9}$$
$$C_6^{3D1} = -\frac{O_{10}}{3} + \frac{10O_{11}}{9} + \frac{2O_{12}}{3} + \frac{8O_{13}}{3} - \frac{O_{14}}{3} + \frac{10O_{15}}{9} + \frac{2O_{16}}{3} + \frac{8O_{17}}{3} + O_7 + \frac{2O_8}{9} + O_9 \quad (29)$$

$$C_1^{3SD1} = -12O_{15} + 12O_{16} + 24O_{17} - 12O_5 - 6O_6 - 6O_7 + 6O_9$$
$$C_2^{3SD1} = -3O_{11} + 3O_{12} + 6O_{13} + 3O_{15} - 3O_{16} - 6O_{17} - 3O_6 - 3O_7 + 3O_9$$
$$C_3^{3SD1} = -5O_{11} - 3O_{12} - 6O_{13} - 2O_{14} - 7O_{15} - O_{16} - 10O_{17} - 6O_5 - 6O_6 - 5O_7 + 2O_8 + 5O_9$$
$$C_4^{3SD1} = -\frac{O_{10}}{2} - 2O_{11} + 2O_{12} + 2O_{13} + \frac{O_{14}}{2} + 2O_{15} - 2O_{16} - 2O_{17} - \frac{3O_6}{2} - \frac{3O_7}{2} + \frac{3O_9}{2}$$
$$C_5^{3SD1} = -12O_6 - 12O_7$$
$$C_6^{3SD1} = -12O_6 - 8O_7 + 4O_8$$
$$C_7^{3SD1} = 3O_{15} - 3O_{16} - 6O_{17}$$
$$C_8^{3SD1} = \frac{O_{14}}{2} + 2O_{15} - 2O_{16} - 2O_{17} - 6O_6 - 6O_7$$
$$C_9^{3SD1} = -6O_6 - 6O_7 + 6O_9$$
$$C_{10}^{3SD1} = -2O_{11} - 6O_{12} - 12O_{13} - 2O_{15} - 6O_{16} - 12O_{17} - 6O_6 - 4O_7 + 2O_8 + 4O_9$$
$$C_{11}^{3SD1} = -6O_6 - 4O_7 + 2O_8$$
$$C_{12}^{3SD1} = -5O_{11} - 3O_{12} - 6O_{13} + O_{15} - 9O_{16} - 18O_{17} - 3O_6 - O_7 + 2O_8 + O_9$$
$$C_{13}^{3SD1} = -2O_{11} - 6O_{12} - 12O_{13} - 2O_{15} - 6O_{16} - 12O_{17} - 3O_6 + 2O_8 \quad (30)$$

$$C^{1D2} = -\frac{2O_{10}}{15} - \frac{8O_{13}}{15} - \frac{2O_{14}}{15} - \frac{8O_{17}}{15} - \frac{2O_7}{15} - \frac{4O_8}{15} - \frac{2O_9}{15}$$
$$C^{3D2} = -\frac{O_{10}}{5} + \frac{2O_{11}}{5} - \frac{2O_{12}}{5} - \frac{O_{14}}{5} + \frac{2O_{15}}{5} - \frac{2O_{16}}{5} - \frac{O_7}{5} - \frac{2O_8}{5} - \frac{O_9}{5}$$
$$C_1^{3P2} = \frac{2O_{10}}{75} + \frac{2O_{11}}{75} - \frac{2O_{12}}{75} + \frac{4O_{13}}{75} + \frac{2O_{14}}{75} + \frac{2O_{15}}{75} - \frac{2O_{16}}{75} + \frac{4O_{17}}{75} + \frac{2O_7}{75} + \frac{4O_8}{75} + \frac{2O_9}{75}$$
$$C_2^{3P2} = \frac{O_{10}}{75} + \frac{2O_{11}}{25} - \frac{2O_{12}}{25} - \frac{8O_{13}}{75} + \frac{O_{14}}{75} + \frac{2O_{15}}{25} - \frac{2O_{16}}{25} - \frac{8O_{17}}{75} + \frac{O_7}{75} + \frac{2O_8}{75} + \frac{O_9}{75}$$
$$C_3^{3P2} = \frac{13O_{10}}{75} + \frac{6O_{11}}{25} - \frac{6O_{12}}{25} + \frac{16O_{13}}{75} + \frac{13O_{14}}{75} + \frac{6O_{15}}{25} - \frac{6O_{16}}{25} + \frac{16O_{17}}{75} + \frac{13O_7}{75} + \frac{26O_8}{75} + \frac{13O_9}{75}$$
$$C^{3F2} = \frac{4O_{10}}{25} + \frac{4O_{11}}{25} - \frac{4O_{12}}{25} + \frac{8O_{13}}{25} + \frac{4O_{14}}{25} + \frac{4O_{15}}{25} - \frac{4O_{16}}{25} + \frac{8O_{17}}{25} + \frac{4O_7}{25} + \frac{8O_8}{25} + \frac{4O_9}{25}$$
$$C_1^{3PF2} = 5O_{11} - 5O_{12} - 10O_{13} + 5O_{15} - 5O_{16} - 10O_{17}$$
$$C_2^{3PF2} = O_{10} + 6O_{11} - 6O_{12} - 8O_{13} + O_{14} + 6O_{15} - 6O_{16} - 8O_{17} + O_7 + 2O_8 + O_9 \quad (31)$$


[1] Y. Xiao, L.-S. Geng, and X.-L. Ren, Phys. Rev. C **99**, 024004 (2019), arXiv:1812.03005 [nucl-th].
[2] E. Epelbaum, W. Gloeckle, and U.-G. Meißner, Nucl. Phys. **A671**, 295 (2000).
[3] D. R. Entem and R. Machleidt, Phys. Rev. **C68**, 041001 (2003).
[4] R. Machleidt and D. R. Entem, Phys. Rept. **503**, 1 (2011).
[5] E. Epelbaum, H. Krebs, and U. G. Meißner, Eur. Phys. J. **A51**, 53 (2015).
[6] E. Epelbaum, H. Krebs, and U.-G. Meißner, Phys. Rev. Lett. **115**, 122301 (2015).
[7] E. Epelbaum, W. Gloeckle, and U.-G. Meissner, Eur. Phys. J. A **19**, 125 (2004), arXiv:nucl-th/0304037.
[8] E. Epelbaum, W. Gloeckle, and U.-G. Meissner, Eur. Phys. J. A **19**, 401 (2004), arXiv:nucl-th/0308010.
[9] E. Epelbaum, W. Glockle, and U.-G. Meißner, Nucl. Phys. **A747**, 362 (2005).
[10] E. Epelbaum, A. M. Gasparyan, J. Gegelia, and H. Krebs, Eur. Phys. J. **A51**, 71 (2015).
[11] Y. Xiao, C.-X. Wang, J.-X. Lu, and L.-S. Geng, Phys. Rev. C **102**, 054001 (2020), arXiv:2007.13675 [nucl-th].
[12] V. G. J. Stoks, R. A. M. Klomp, M. C. M. Rentmeester, and J. J. de Swart, Phys. Rev. **C48**, 792 (1993).
[13] R. Machleidt, K. Holinde, and C. Elster, Phys. Rept. **149**, 1 (1987).
[14] S. Shen, H. Liang, W. H. Long, J. Meng, and P. Ring, Prog. Part. Nucl. Phys. **109**, 103713 (2019), arXiv:1904.04977 [nucl-th].
[15] R. Navarro Pérez, J. E. Amaro, and E. Ruiz Arriola, Phys.

Rev. C **88**, 024002 (2013), [Erratum: Phys.Rev.C 88, 069902 (2013)], arXiv:1304.0895 [nucl-th].
[16] R. Navarro Pérez, J. E. Amaro, and E. Ruiz Arriola, Phys. Rev. C **91**, 054002 (2015), arXiv:1411.1212 [nucl-th].
[17] R. Navarro Pérez, J. E. Amaro, and E. Ruiz Arriola, Phys. Rev. C **95**, 064001 (2017), arXiv:1606.00592 [nucl-th].
[18] A. G. Escalante, R. Navarro Pérez, and E. Ruiz Arriola, Phys. Rev. C **104**, 054002 (2021), arXiv:2010.03885 [nucl-th].
[19] R. J. Furnstahl, N. Klco, D. R. Phillips, and S. Wesolowski, Phys. Rev. C **92**, 024005 (2015), arXiv:1506.01343 [nucl-th].
[20] J. A. Melendez, S. Wesolowski, and R. J. Furnstahl, Phys. Rev. C **96**, 024003 (2017), arXiv:1704.03308 [nucl-th].
[21] J. A. Melendez, R. J. Furnstahl, D. R. Phillips, M. T. Pratola, and S. Wesolowski, Phys. Rev. C **100**, 044001 (2019), arXiv:1904.10581 [nucl-th].
[22] E. Epelbaum et al., Eur. Phys. J. A **56**, 92 (2020), arXiv:1907.03608 [nucl-th].
[23] E. Epelbaum, H. Krebs, and P. Reinert, Front. in Phys. **8**, 98 (2020), arXiv:1911.11875 [nucl-th].
[24] P. Maris et al., Phys. Rev. C **103**, 054001 (2021), arXiv:2012.12396 [nucl-th].
